# Supplementary material for: The Missing Link: Finding label relations across datasets
Source: arXiv:2206.04453 source file (2022-08-09)
Supplement: Supplementary file 1 [file 9_appendix.tex]

\input{4_2_ILSVRC_COCO}
\input{5_4_benefit_for_knowledge_transfer}
